# Supplementary material for: Beyond Sharing: Conflict-Aware Multivariate Time Series Anomaly Detection
Source: arXiv:2308.08915 source file (2023-08-25)
Supplement: Supplementary file 1 [file appendix.tex]

\appendix
\section{Datasets Details}
\label{app: data}
% The summary of these datasets is listed in Table \ref{table.data}, including the number of entities, dataset size, the number of dimensions and anomaly ratio in the test set.
% \begin{table}[htb]
% \caption{Dataset Statistics.}
% \begin{tabular}{cccccc}
% \toprule
% Dataset & Entities & Metrics & Train  & Test   & Anomaly (\%) \\ \hline
% SMD     & 28       & 38         & 708405 & 708420 & 4.16        \\
% SWaT    & 1        & 51         & 495000 & 449919 & 11.98       \\
% WADI    & 1        & 123        & 784517 & 172801 & 5.77        \\ 
% \bottomrule
% \end{tabular}
% \label{table.data}
% \end{table}

\textit{Server Machine Dataset (SMD)}. SMD is collected from a large Internet company and published on GitHub, whose observations are equally-spaced 1 minute apart~\cite{omni}. It includes time series of 28 machines distributed in three clusters. Each machine is pre-divided into a training set and a test set. Both of them contain 38 metrics. Anomalies in the test set are labeled by domain experts.

\textit{Secure Water Treatment (SWaT)}. SWaT is collected from a real-world water treatment plant, recording 11 days of continuous operation, 7 days under normal operation and 4 days with attack scenarios. Metrics are collected by 51 sensors and actuators. As two versions of the training set are available on the official website, we select the latest Version 1.

\textit{Water Distribution (WADI)}. WADI is an extension of the SWaT testbed with 123 sensors and actuators. Data under 14 days of normal operations are recorded as the training set, and data under attacks within 2 days are recorded as the test set. We use the latest CSV file "WADI\_14days\_new.csv" given by the official website as the training set, which removes readings affected by certain unstable periods.

% \section{Experiment Settings}
\section{Experimental Environment}
CAD and other PyTorch-based methods run on a machine equipped with two Intel(R) Xeon(R) Silver 4316 CPUs and one NVIDIA GeForce RTX 3090 24GB GDDR6 GPU. Since the driver of RTX 3090 is not compatible with CUDA 10.2 and previous versions, methods implemented in TensorFlow 1.x and TensorFlow 2.0 are performed on one NVIDIA Tesla K80 core with 12GB GDDR5 memory.
